# Supplementary material for: ProgramAlly: Creating Custom Visual Access Programs via Multi-Modal End-User Programming
Source: arXiv:2408.10499 source file (2024-08-20)
Supplement: Supplementary file 1 [file 10_appendix.tex]

\clearpage 

%(Push text down one more page)
%\clearpage

\section{\sys's Item and Adjective Types}

\add{Here, for reproducibility, we list the item and adjective types available in \sys, along with their source models if applicable.}

\add{
\textbf{Object Types:} \sys uses default YOLO and customized YOLO-world models for object detection.
Initially \sys used the 80 COCO object classes detected by YOLOv8.
However, through our formative design research, we knew that these classes were not sufficient for tasks that blind people would need to do. To add additional classes, we used a set of YOLO-world models which can add new classes without training \cite{yolo-world}.
While these models currently present a significant loss of accuracy, we found that we were able to balance this by limiting the number of classes added to each model, and particularly avoiding class labels that could be easily confused for each other. Through testing various combinations of classes heuristically, this resulted in four additional models: 
\begin{itemize}
    \item An outdoor navigation model (`sign', `license plate'),
    \item An indoor navigation model (`door', `stairs', `hallway', `exit sign', `trash can'),
    \item A reading model (`envelope', `package', `document', `poster'),
    \item And a product identification model (`package', `can', `bottle', `box', `product', `jar'). This model suffers from the issue of similar class labels being misidentified (i.e., a jar is often labeled as a can and vice versa). Because of this, we created an umbrella class for these labels called ``grocery product'' that achieves coverage over the product types mentioned while disregarding mislabels.
\end{itemize}
}

\add{
\textbf{Text Types:} \sys detects text with iOS's native text recognition. The base text type `any text' returns any string where the majority of the bounding box is contained within the parent object. 
\sys can then filter these strings for different types of text in one of two ways:
\begin{itemize}
    \item RegEx Functions: `number', `time', `date'
    \item Google’s Entity Extraction API: `address', `email', `flight number', `IBAN', `ISBN', `money', `credit card number', `US phone number', `tracking number', `URL'  
\end{itemize}
}

\add{
\textbf{Property Types:} \sys also allows two `properties' to be used as items within programs: `color' and `count'. For example, \texttt{`find COLOR on CAR'} or \texttt{`find COUNT on BOOK'} (with the latter being better represented in natural language as `find number of books'; this was not used in our evaluation so the particular syntax is clunky and could be improved in the future).
}

\add{
\textbf{Adjective Types:} \sys includes the following three adjective types:
\begin{itemize}
    \item Colors (most frequent pixel colors in object bounding box mapped to strings): `black', `dark gray', `light gray', `white', `gray', `red', `green', `blue', `cyan', `yellow', `magenta', `orange', `purple', `brown'
    \item Location (quadrant on parent item): `lower left', `center lower', `lower right', `left middle', `center middle', `right middle', `upper left', `lower center', `upper right'
    \item Size (relative to items of the same type in the same parent item): `largest', `smallest'
\end{itemize}
}

\section{\sys's Natural Language Mode Prompts}

\add{
Here, we include our full system prompt to GPT-4 for converting natural language queries into programs. This includes approximately 20 examples as few-shot `training data'. In an attempt to reduce hallucination for new object types, we used GPT-4's `function calling' feature, wherein a function specification can be provided to the model and it will attempt to respond with JSON that provides parameters to call that function.
}

\small
\begin{lstlisting}[language=json, caption=Custom function specification for GPT-4.]
interpret_object_query_function = {
"name": "interpret_object_query",
"description": "Interprets queries about specified objects, and optionally their attributes. Attributes must be paired with an object.",
"parameters": {
    "type": "object",
    "properties": { "query_items": {
        "type": "array",
        "description": "A list of object targets with an optional descriptor, from most to least specific. If no close match is found, use 'any object'.",
        "items": {
            "type": "object",
            "properties": {
                "object": {
                    "type": "string", 
                    "enum": [list of all program items] 
                },
                "descriptor": {
                    "type": "string", 
                    "enum": [all program adjectives] 
                },
        }, }, 
    }, },
    "required": [ "query_items" ]
}, }
\end{lstlisting}

\begin{lstlisting}[language=json, firstnumber=1, caption=System message.]
system_message = [{
    "role": "system", 
    "content": "Use the interpret_object_query function to interpret questions about objects."
}]
\end{lstlisting}

\begin{lstlisting}[language=json, firstnumber=1, caption=Chat history as few-shot training data. Includes original requests and modifications.]
{ "role": "user", "content": "What is the license plate number of this car?" },
{
    "role": "assistant",
    "content": '{ "query": [ [ {"object": "any text"}, {"object": "license plate"}, {"object": "car"} ] ] }'
},  
{ "role": "user", "content": "Modify the previous program: Also read out the color of the car" },
{
    "role": "assistant",
    "content": '{ "query": [ [ {"object": "any text"}, {"object": "license plate"}, {"object": "car"} ], [ {"object": "color"}, {"object": "car"} ] ] }'
}, 
{ "role": "user", "content": "What is the license plate number of the black car?" },
{
    "role": "assistant",
    "content": '{ "query": [ [ {"object": "any text"}, {"object": "license plate"}, {"descriptor": "black", "object": "car"} ] ] }'
},
{ "role": "user", "content": "Read the expiration date on these products." },
{
    "role": "assistant",
    "content": '{ "query": [ [ {"object": "date"}, {"object": "grocery product"} ] ] }'
},
{ "role": "user", "content": "Modify the previous program: Add the product names." },
{
    "role": "assistant",
    "content": '{ "query": [ [ {"object": "date"}, {"object": "grocery product"} ], [ {"descriptor": "largest", "object": "any text"}, {"object": "grocery product"} ] ] }'
},
{ "role": "user", "content": "What is the color of the text on the bus?" },
{
    "role": "assistant",
    "content": '{ "query": [ [ {"object": "color"}, {"object": "any text"}, {"object": "bus"} ] ] }'
},
{ "role": "user", "content": "How many people are sitting on this bench?" },
{
    "role": "assistant",
    "content": '{ "query": [ [ {"object": "count"}, {"object": "person"}, {"object": "bench"} ] ] }'
},
{ "role": "user", "content": "What is the orange text on this envelope?" },
{
    "role": "assistant",
    "content": '{ "query": [ [ {"descriptor": "orange", "object": "any text"}, {"object": "envelope"} ] ] }'
},
{ "role": "user", "content": "What is the route of this bus?" },
{
    "role": "assistant",
    "content": '{ "query": [ [ {"object": "number"}, {"object": "bus"} ] ] }'
},
{ "role": "user", "content": "Modify the previous program: Only for blue busses" },
{
    "role": "assistant",
    "content": '{ "query": [ [ {"object": "number"}, {"descriptor": "blue", "object": "bus"} ] ] }'
},
{ "role": "user", "content": "What does this bottle say?" },
{
    "role": "assistant",
    "content": '{ "query": [ [ {"object": "any text"}, {"object": "grocery item"} ] ] }'
},
{ "role": "user", "content": "Modify the previous program: Just say the biggest text" },
{
    "role": "assistant",
    "content": '{ "query": [ [ {"descriptor": "largest", "object": "any text"}, {"object": "grocery item"} ] ] }'
},
{ "role": "user", "content": "What is the text in the middle of this envelope?" },
{
    "role": "assistant",
    "content": '{ "query": [ [ {"object": "any text"}, {"descriptor": "center middle", "object": "envelope"} ] ] }'
},
{ "role": "user", "content": "Modify the previous program: What's in the top left?" },
{
    "role": "assistant",
    "content": '{ "query": [ [ {"object": "any text"}, {"descriptor": "top left", "object": "any object"} ] ] }'
},
{ "role": "user", "content": "What tempurature is my oven set to?" },
{
    "role": "assistant",
    "content": '{ "query": [ [ {"object": "number"}, {"object": "oven"} ] ] }'
},
{ "role": "user", "content": "What is my oven set to?" },
{
    "role": "assistant",
    "content": '{ "query": [ [ {"object": "number"}, {"object": "oven"} ] ] }'
},
{ "role": "user", "content": "What is the time on my microwave?" },
{
    "role": "assistant",
    "content": '{ "query": [ [ {"object": "time"}, {"object": "microwave"} ] ] }'
},
{ "role": "user", "content": "Is this table empty?" },
{
    "role": "assistant",
    "content": '{ "query": [ [ {"object": "any object"}, {"object": "dining table"} ] ] }'
},
{ "role": "user", "content": "Modify the previous program: Are my keys here?" },
{
    "role": "assistant",
    "content": '{ "query": [ [ {"object": "keys"}, {"object": "dining table"} ] ] }'
},
\end{lstlisting}

\section{\sys's Full Study Protocol}
\label{chpt:appendix_04_PAprotocol}

\subsection{Pre-Study Demographics Form}
\begin{enumerate}
    \item Gender (short text).
    \item Age.
    \item Occupation (short text).
    \item Describe your level of vision (long text).
    \item At what age did you experience vision loss (long text).
    \item Describe your level of hearing (long text).
    \item Which screen readers do you regularly use (NVDA, JAWS, VoiceOver, Talk Back, Other).
\end{enumerate}

\subsection{User Study (Approximately 2 Hours)}

\subsubsection{Assistive Technology Background Interview}

\begin{enumerate}
    \item Do you use any camera-based assistive applications on your phone, like Be My Eyes, or Seeing AI?
    \item How do you feel about the feedback you receive from Seeing AI? Do you feel like you ever deal with information overload?
    \item How often do you try new technologies? This could be assistive technology, or other new software and devices.
    \item Do you have any experience programming?
\end{enumerate}

\subsubsection{\sys Set-Up and Tutorial}

\textit{The purpose of this application is to let you create personalized filters for visual information. So the app will scan things around you with the camera, and you can set up filters for certain pieces of information that you might be looking for. 
So for an example of filtering visual information, you could use this app to specify a certain type of text that you’re looking for or certain objects, and have it only speak out that type of information.
In the app I’ll have you test out, you will create these filters by writing short 
by writing short programs to specify exactly what you want to hear. And I’ll explain more about how to do this as we go through the study, so don’t worry about it yet.
}

\begin{enumerate}
    \item Open an existing program from the pre-made library, for example, \texttt{`find NUMBER on BUS'}.
    \begin{enumerate}
        \item What do you think this program would do?
        \item What other thoughts did you have while reading through this page?
    \end{enumerate}

    \item Run the example program, either with a sample image or a prop.
    \begin{enumerate}
        \item What did you think while running this program? Did the output match your expectations?
        \item Do you feel like this is something you could use in your daily life? What is your current strategy for doing this task? How did it compare with Seeing AI/ Be My AI?
        \item What do you think about the amount of information that you heard from the program? Was it too much or too little? Was there anything else you wanted to hear?
        \item Do you have any other thoughts about this program that you would like to share?
    \end{enumerate}

    \item Practice modifying the example program by adding an adjective, for example, \texttt{`find NUMBER on RED BUS'}
    \begin{enumerate}
        \item What thoughts did you have while modifying this page?
    \end{enumerate}
\end{enumerate}

\subsubsection{Program Creation Tasks}

For each of the three program creation modes, participants followed the protocol below. Participants were first given a brief verbal description of the program creation mode:

\begin{itemize}
    \item \textbf{Block Mode:} \textit{``The first way that you can create programs is by setting up the filters directly. So just like in the page that you read through at first with the Expiration Date program.''}
    \item \textbf{Explore Mode:} \textit{``The next way that you can create a program is by generating a program from an example image or video. The app will list out all of the pieces of information that you might want to find in an image, and it will generate a program that filters for that information next time.''}
    \item \textbf{Question Mode:} \textit{``The last way that you can create a program is by asking a question out loud, and the app will generate a program based on the question.''}
\end{itemize}

\begin{enumerate}
    \item Create a new program from a prompt, for example, \textit{``I want you to try creating a program that will find the route number on a bus.''}
    \begin{enumerate}
        \item Can you describe the program that you just created? What do you think this would do?
        \item What other thoughts did you have while creating this program?
        \item From a scale of 1 to 7, how much do you agree with `It was easy to create this program'? Why? 
        \item From a scale of 1 to 7, how much do you agree with `This program is correct'? Why? 
        \item If you could edit this program, what would you change to make it more correct?
    \end{enumerate}

    \item If successful, run the created program, either on an example image or a prop.
    \begin{enumerate}
        \item What did you think while running this program? Did the output match your expectations?
        \item Do you feel like this is something you could use in your daily life? What is your current strategy for doing this task? How did it compare with Seeing AI/ Be My AI?
        \item What do you think about the amount of information that you heard from the program? Was it too much or too little? Was there anything else you wanted to hear?
        \item Do you have any other thoughts about this program that you would like to share?
    \end{enumerate}

    \item (In-person participants only) Compare doing the same task with Seeing AI or Be My AI. What are the pros and cons of each?

    \item (Question mode only) Modify the program slightly by asking a follow-up question.
    \begin{enumerate}
        \item Did this produce the program you expected?
        \item What did you think about editing the program this way?
        \item What other thoughts did you have while modifying the program this way?
    \end{enumerate}
    
\end{enumerate}

\subsubsection{Comparing Creation Modes}

\begin{enumerate}
    \item Rank three modes from overall favorite to least favorite.
    \item Rank three modes from the most to least effort.
    \item Rank the three modes from the most to least accurate.
    \item What are the pros and cons of each mode?
\end{enumerate}

\subsubsection{Comparing with Other Technologies (In-Person Only)}

In-person participants also tried the program \texttt{`find LARGEST TEXT on POSTER'}, and compared it to Seeing AI and/ or Be My AI.

\subsubsection{Open-Ended Interview}

\begin{enumerate}
    \item If you could create a new filtering program, what would it be?
    \item What did you think of this app overall?
    \item Is this something that you can see you using out in the real world? Would you want to add anything to the app to be able to use it in your day to day life? How would it fit into your current assistive technology workflow?
    \item In this app, you created filters that you could then save, and re-use in different situations. I’m curious what you think about the effort of creating these filters versus the potential benefit? Can you imagine making different filters to open and use when you need them?
    \item We wanted to see how this app could help people customize assistive technology. And it helps customize filters for information. Do you think this type of customization could be applied to other things? Are there other things you would like to customize? What are the benefits of customizations?
    \item Is there anything else that you would like to add that you did not get a chance to yet?
\end{enumerate}

\subsubsection{Program Tasks and Props}

Programs and props for in-person study participants:
\begin{enumerate}
    \item Tutorial program: \texttt{find NUMBER on BUS}, Example image of red bus
    \item Modify tutorial program: \texttt{find NUMBER on RED BUS}, No prop
    \item Create w/ blocks: \texttt{find ADDRESS on PACKAGE}, Packages and letters
    \item Create w/ explore: \texttt{find TEXT on BOOK}, Various books
    \item Create w/ question: \texttt{find DATE on GROCERY ITEM}, Canned/ dry goods
    \item Modify w/ question: \texttt{find DATE on GROCERY ITEM}, changed to \texttt{find TEXT on GROCERY ITEM}, No prop    
    \item Compare w/ other apps:  \texttt{find LARGEST TEXT on POSTER}, Printed event posters
\end{enumerate}

Programs and tasks for remote study participants:
\begin{enumerate}
    \item Tutorial program: \texttt{find NUMBER on BUS}, Example image of red bus
    \item Modify tutorial program: \texttt{find NUMBER on RED BUS}, No sample image
    \item Create w/ blocks: \texttt{find PERSON on BENCH}, Image of bench with two people 
    \item Create w/ explore: \texttt{find TEXT on BOOK}, Image of `Of Mice and Men'
    \item Create w/ question: \texttt{find DATE on GROCERY ITEM}, Image of milk carton with date
    \item Modify w/ question: \texttt{find DATE on GROCERY ITEM} changed to \texttt{find TEXT on GROCERY ITEM}, No sample image
\end{enumerate}
